# Supplementary material for: Generative Recommendation: Towards Next-generation Recommender Paradigm
Source: arXiv:2304.03516 source file (2024-02-25)
Supplement: Supplementary file 1 [file 6_SI.tex]

\section{Appendix}
\label{sec:appendix}
